# Supplementary material for: Optically driving the radiative Auger transition
Source: arXiv:2105.03447 source file (2021-05-07)
Supplement: Supplementary file 1 [file supplement.pdf]

# Supplement for "Optically driving the radiative Auger transition"

Clemens Spinnler[1,*], Liang Zhai[1,*], Giang N. Nguyen[1], Julian Ritzmann[2], Andreas D. Wieck[2], Arne Ludwig[2], Alisa Javadi[1], Doris E. Reiter[4], Paweł Machnikowski[3], Richard J. Warburton[1], and Matthias C. Löbl[1,*,†]

[1]*Department of Physics, University of Basel, Klingelbergstrasse 82, 4056 Basel, Switzerland*
[2]*Lehrstuhl für Angewandte Festkörperphysik, Ruhr-Universität Bochum, 44780 Bochum, Germany*
[3]*Department of Theoretical Physics, Wrocław University of Science and Technology, 50-370 Wrocław, Poland*
[4]*Institut für Festkörpertheorie, Universität Münster, 48149 Münster, Germany*

[*] *These authors contributed equally to this work.*
[†] *Correspondence should be addressed to: matthias.loebl@unibas.ch*

## I. MODELLING THE Λ-SYSTEM

The level scheme for our two-laser experiments is shown in Fig. 1. It consists of the electron ground state $|s\rangle$, an excited electron state $|p\rangle$, and the trion state $|t\rangle$. The laser on the fundamental transition is labelled as $\omega_1$ and the laser on the radiative Auger transition is labelled as $\omega_2$. The corresponding Rabi frequencies are given by $\Omega_1$, $\Omega_2$ and the detunings of the lasers from the corresponding transition are $\Delta_1$, $\Delta_2$. The spontaneous decay rates are the decay rate via the fundamental transition ($\Gamma_r$), the decay rate via radiative Auger ($\Gamma_A$), and the $p$-to-$s$ decay rate ($\Gamma_p$). We simulate the system with a standard quantum optics approach. Making the dipole and the rotating-wave approximations, the Hamiltonian of the system is given by[1,2]:

$$\hat{H} = \frac{\hbar}{2}[2(\Delta_2 - \Delta_1)\,|p\rangle\langle p| - 2\Delta_1\,|t\rangle\langle t| + \Omega_1\,|t\rangle\langle s| + \Omega_2\,|t\rangle\langle p| + \Omega_1\,|s\rangle\langle t| + \Omega_2\,|p\rangle\langle t|] \quad (1)$$

The Hamiltonian describes the coherent evolution of the system. The incoherent decay paths are taken into account by the Lindblad collapse operators for the spontaneous emission from the fundamental transition ($L_1 = \sqrt{\Gamma_r}\,|s\rangle\langle t|$), the spontaneous radiative Auger emission ($L_2 = \sqrt{\Gamma_A}\,|p\rangle\langle t|$)), and the $p$-to-$s$ relaxation ($L_3 = \sqrt{\Gamma_p}\,|s\rangle\langle p|$)). The dynamics of the system is described by the following master equation:

$$i\hbar\frac{d\rho}{dt} = [\hat{H},\rho] + i\hbar\sum_i\left(L_i\rho L_i^\dagger - \frac{1}{2}\{L_i^\dagger L_i,\rho\}\right), \quad (2)$$

where $\rho$ is the density matrix of the system. Using this equation, we determine the steady state of the system ($\frac{d\rho}{dt} = 0$). The steady state occupation of the trion state is used for simulating the experiments as it is proportional to the fluorescence intensity.

This quantum optics simulation fits well to our experimental results in Fig. 3 of the main text. We also use it to estimate the Rabi frequency $\Omega_2$ and the dephasing $\gamma_p$: when $\Delta_2$ between laser and transition is close to zero, the resonance fluorescence changes depending on $\Omega_2$. Due to the small dipole moment of the radiative Auger transition, strong laser powers are required to achieve high values for $\Omega_2$. For the strongest laser power of $\omega_2$ (increasing the power of $\omega_1$ by a factor of $\sim 8\times10^3$), we estimate $\Omega_2 = 2\pi\times3.2$ GHz from the quantum optics simulation. Alternatively, one could estimate the ratio of the corresponding dipole moments by using the intensity ratio between resonance fluorescence and radiative Auger emission ($\sim 50:1$). $\Omega_2$ could then be obtained by using this estimation together with the power saturation curve of the resonance fluorescence. We find that this method underestimates $\Omega_2$ compared to the quantum optics simulation. Since effects such as chromatic aberration make this second approach more prone to systematic errors, we always use the two-laser experiment and the corresponding quantum optics simulation to determine $\Omega_2$. The

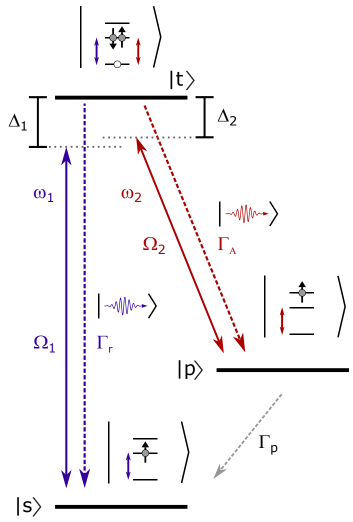


FIG. 1. **The level scheme.** Fundamental transition and radiative Auger transition form a Λ-system where both transitions can be driven by two independent lasers. The Rabi-frequency of the laser on the fundamental transition ($\omega_1$) is given by $\Omega_1$, the Rabi frequency of the laser on the radiative Auger transition ($\omega_2$) is given by $\Omega_2$. The corresponding laser detunings are $\Delta_1$ and $\Delta_2$, the corresponding spontaneous decay rates are $\Gamma_1$, $\Gamma_2$. The parameter $\Gamma_p$ is the relaxation rate from the electron excited state $|p\rangle$ to the electron ground state $|s\rangle$.

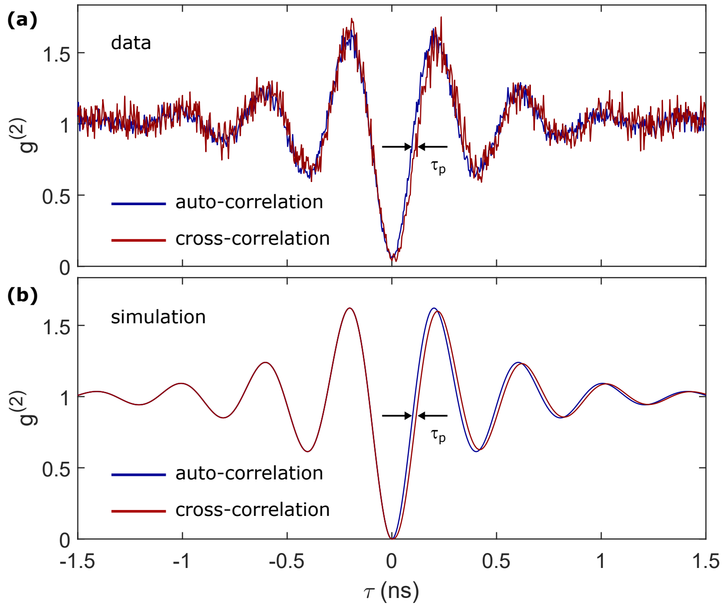


FIG. 2. **Auto- and cross-correlation experiments (a)** Experimental data for the auto-correlation of the fluorescence from the fundamental transition and the cross-correlation between fluorescence from the fundamental transition and radiative Auger. **(b)** Simulation of the correlation measurements. The $p$-to-$s$ relaxation time is determined from these fits to be $\tau_p = 17$ ps.

dephasing term $\gamma_p$ is also estimated by simulating the two-laser experiment. We find that it mainly affects the width of the fluorescence dip. As explained in the main text, other parameters ($\Gamma_r$, $\Gamma_p$, $\Omega_1$) are determined from independent measurements and kept fixed in the simulation.

## II. MODEL FOR CORRELATION MEASUREMENTS

Time-resolved correlation measurements ($g^{(2)}$-measurements) are used to determine the relaxation time $\tau_p = 1/\Gamma_p$. An auto-correlation of the resonance fluorescence from the fundamental transition and a cross-correlation between emission from the fundamental transition and radiative Auger emission are shown in Fig. 2(a). As shown in Fig. 2(b), the theoretical model fits well to the data. In these measurements, only a single laser at $\omega_1$ is used. The system is described by Eqs. 1 and 2, with the parameter $\Omega_2$ set to zero. We use the Quantum Toolbox in Python (QuTiP[3]) to compute the steady state density matrix. With the resulting density matrix, we then compute the auto- and the cross-correlation. The auto-correlation is:

$$g^{(2)}(\tau) = \frac{\langle \hat{a}^\dagger(t)\hat{a}^\dagger(t+\tau)\hat{a}(t+\tau)\hat{a}(t)\rangle}{\langle \hat{a}^\dagger(t)\hat{a}(t)\rangle^2}, \quad (3)$$

and the cross-correlation is:

$$g^{(2)}(\tau) = \frac{\langle \hat{a}_A^\dagger(t)\hat{a}^\dagger(t+\tau)\hat{a}(t+\tau)\hat{a}_A(t)\rangle}{\langle \hat{a}^\dagger(t)\hat{a}(t)\rangle\langle \hat{a}_A^\dagger(t)\hat{a}_A(t)\rangle}. \quad (4)$$

In both cases, $t$ is the time and $\tau$ is the time delay between two subsequently detected photons. $\hat{a}^\dagger$ describes the decay into the $s$-shell (fundamental transition), and $\hat{a}_A^\dagger$ describes the radiative Auger decay into the excited electron state, $|p\rangle$.

## III. MAGNETIC FIELD DISPERSION OF THE EMISSION

The magnetic field dispersion of the radiative Auger emission is significantly stronger than that of the emission from the fundamental transition. The reason is the different final state after the optical decay: the electron ground state $|s\rangle$ ($s$-shell) has a weak magnetic field dispersion and, in contrast, higher shells such as the excited state $|p\rangle$ ($p$-shell) have a much stronger dependence on the magnetic field. Since the optical emission energy is given by the energy of the trion minus the energy of the final state, the strong magnetic field dispersion is transferred to the radiative Auger lines. The strong dispersion of the radiative Auger emission is an important feature allowing it to be distinguished unambiguously from phonon replicas. For a two-dimensional harmonic confinement potential, the magnetic field dispersions of the different shells form the Fock-Darwin spectrum[4]. The dispersion of the radiative Auger emission is, therefore, typically close to an inverted Fock-Darwin spectrum[5]. A model for the magnetic field dispersion has been developed in Ref. 5.

[1] M. Fleischhauer, A. Imamoglu, and J. P. Marangos, Rev. Mod. Phys. **77**, 633 (2005).

[2] J. H. Prechtel, J. H. A. V. Kuhlmann, A. Ludwig, S. R. Valentin, A. D. Wieck, and R. J. Warburton, Nat. Mater. **15**, 981 (2016).

[3] J. R. Johansson, P. D. Nation, and F. Nori, Comput. Phys. Commun. **184**, 1234 (2013).

[4] L. P. Kouwenhoven, D. G. Austing, and S. Tarucha, Rep. Prog. Phys. **64**, 701 (2001).

[5] M. C. Löbl, C. Spinnler, A. Javadi, L. Zhai, G. N. Nguyen, J. Ritzmann, L. Midolo, P. Lodahl, A. D. Wieck, A. Ludwig, and R. J. Warburton, Nat. Nanotechnol. **15**, 558 (2020).
